# Supplementary material for: Modelling cell-cell collision and adhesion with the Filament Based Lamellipodium Model
Source: arXiv:1809.07852 source file (2018-09-20)
Supplement: Supplementary file 1 [file A_appendix.tex]

%!TeX root =main.tex
%------------------------------------------------------------------------------
\section{The FEM that solves the FBLM}
The numerical solution of the FBLM \eqref{eq:strong} follows from a problem specific FEM that was first presented in  \cite{MOSS-numeric}. Here we address some of its components.

The maximal filament length $L(\a,t)$ varies with $\a$ all around the lamellipodium; the computational domain 
\[
	B(t) = \left\{(\alpha,s):\, 0\le\a<2\pi\,,\, -L(\alpha,t)\le s < 0\right\}
\]
is non-rectangular.  For consistency and stability reasons we recover the orthogonality of the domain $B(t)$, using the coordinate transformation 
\[
	(\alpha,s,t) \rightarrow \(\alpha, L(\alpha,t)s, t\) \,,
\]
and replace it by
\begin{equation}\label{eq:rescaled.B}
B_0 := [0,2\pi)\times[-1,0)\ni (\alpha,s)\,.
\end{equation}
%\begin{figure}[t]
%	\centering 	
%	\begin{tabular}{ccc}
%		{\includegraphics[height=12em]{input/DisretizedCell.pdf}}
%		&&{\includegraphics[height=10em]{input/IndexedCellPart.pdf}}\\
%		\footnotesize{(a)} && \footnotesize{(b)}
%	\end{tabular}
%	\caption{A rotational symmetric lamellipodium along with the projection of both families of discretization filaments of the domain $B_0$. In (a) are shown the ``discretization filaments'' of the complete lamellipodium, and in (b) a lamellipodium fragment detail with the enumeration of the filaments and of the discretization cells.}\label{fig:discr}
%\end{figure}

Accordingly, the weak formulation of (\ref{eq:strong}), recasts into
\begin{align}
0 	=&\int_{B_0}\eta \left( \mu^B \partial^2_s\vec{F} \cdot \partial_s^2\vec{G} + L^4\mu^A \widetilde{D_t} \vec{F} \cdot \vec{G} + L^2\lambda_\text{inext} \partial_s\vec{F} \cdot \partial_s\vec{G} \right) d(\alpha,s) \nonumber\\
&+\int_{B_0}  \eta\eta^*\left( L^4\widehat{\mu^S} \(\widetilde{D_t}\vec{F}  - \widetilde{D_t^*}\vec{F}^* \)\cdot \vec{G} \mp L^2\widehat{\mu^T}(\phi-\phi_0)\partial_s\vec{F}^{\perp} \cdot \partial_s \vec{G} 
\right) \ d(\alpha,s) \nonumber\\
&- \int_{B_0} p(\varrho) \left( L^3\partial_\a \vec{F}^{\perp}\cdot \partial_s \vec{G} - \frac{1}{L}\partial_s \vec{F}^{\perp}\cdot \partial_\a (L^4\vec{G})\right) d(\alpha,s) \nonumber\\
&+	\int_0^{2\pi} \eta \left( L^2 f_\text{tan}\partial_s\vec{F} + L^3 f_{\text{inn}}\vec{V} \right)\cdot \vec{G} \Bigm|_{s=-1}d\a \mp	\int_0^{2\pi} L^3\lambda_\text{tether}\nu\cdot \vec{G} \Bigm|_{s=0} d\a \,,\label{eq:FEM}
\end{align}
with $\vec{F}, \vec{G}\in H^1_\a\((0,2\pi);\,H^2_s(-1,0)\)$. In a similar manner the modified material derivative and in-extensibility conditions read 
\[
	\widetilde{D_t} = \partial_t - \(\frac{v}{L} + \frac{s \partial_t L}{L}\)\partial_s
\]
and
\[
	\left|\partial_s \mathbf F(\alpha,s,t)\right| = L(\alpha,t).
\]

We decompose $B_0$ into disjoined rectangular \textit{computational cells} as follows:
\begin{equation}\label{eq:cell}
B_0 = \bigcup_{i=1}^{N_a} \bigcup_{j=1}^{N_s -1} C_{i,j} \,,\quad
\mbox{where}\quad  C_{i,j}=[\alpha_i,\alpha_{i+1})\times[s_j,s_{j+1}) \,,
\end{equation}
for $\alpha_i = (i-1)\Delta \alpha$, $\Delta \alpha = \frac{2\pi}{N_\a}$, $i = 1,\ldots,N_\a+1$, and $s_j = -1 + (j-1)\Delta s$, $\Delta s = \frac{1}{N_s - 1}$, $j = 1,\ldots,N_s$. The resolution of the grid along the $\a$ and $s$ directions is denoted by $\anodes$, $\snodes$. The $\a$-periodicity assumption suggests that $\alpha_{N_\a+1} = 2\pi$ is identified with $\alpha_1 = 0$.%, see also Figure \ref{fig:discr}.

We follow \cite{MOSS-numeric} and set the conforming FE space
\begin{align}
\mathcal V := \Bigl\{ \vec{F}\in C_\a&\([0,2\pi];\, C^1_s([-1,0])\)^2 \text{ such that } \vec{F}\bigm|_{C_{i,j}}(\cdot,s) \in \mathbb{P}^1_\a\,,\, \nonumber \\
&\vec{F}\bigm|_{C_{i,j}}(\a,\cdot) \in \mathbb{P}^3_s\quad\mbox{for } i=1,\ldots,N_\a\,;\,  j = 1,\ldots,N_s-1\Bigr\}  \,, \label{eq:FE:V}
\end{align}
of continuous functions that are continuously differentiable with respect to $s$, and such that on each computational cell they coincide with a first order polynomial in $\a$, and a third order polynomial in $s$.

%\begin{figure}[t]
%	\centering
%	\begin{tabular}{cccc}
%		{\includegraphics[width=0.21\textwidth]{input/H1.pdf}}&
%		{\includegraphics[width=0.21\textwidth]{input/H2.pdf}}&
%		{\includegraphics[width=0.21\textwidth]{input/H3.pdf}}&
%		{\includegraphics[width=0.21\textwidth]{input/H4.pdf}}\\
%		\footnotesize{(a) $H_1^C$} & \footnotesize{(b) $H_1^C$} & \footnotesize{(c) $H_1^C$} & \footnotesize{(d) $H_1^C$}
%	\end{tabular}
%	\caption{Graphical representation of four of the Lagrange-Hermite shape functions (\ref{eq:H}) over the generic discretization cell $C$. The $H_1^C$, $H_3^C$, $H_5^C$, and $H_7^C$ attain the value 1 and the derivative 0 at the corners of $C$,  whereas the rest attain the value 1 and derivative 0 at the corners of $C$.}\label{fig:shape}
%\end{figure}

In particular, we consider for $i = 1,\ldots,N_\a+1$, $i = j,\ldots,N_s$, and  $(\a,s)\in C_{i,j}$,  that
\begin{equation}\label{eq:H}
\left\{ \begin{array}{lcl}
H_1^{i,j}(\a,s)=L_1^{i,j}(\a) G_1^{i,j}(s),&~& 
H_5^{i,j}(\a,s)=L_2^{i,j}(\a) G_1^{i,j}(s)\\
H_2^{i,j}(\a,s)=L_1^{i,j}(\a) G_2^{i,j}(s),&& 
H_6^{i,j}(\a,s)=L_2^{i,j}(\a) G_2^{i,j}(s)\\
H_3^{i,j}(\a,s)=L_1^{i,j}(\a) G_3^{i,j}(s),&& 
H_7^{i,j}(\a,s)=L_2^{i,j}(\a) G_3^{i,j}(s)\\
H_4^{i,j}(\a,s)=L_1^{i,j}(\a) G_4^{i,j}(s),&& 
H_8^{i,j}(\a,s)=L_2^{i,j}(\a) G_4^{i,j}(s) 
\end{array}\right.
\end{equation}
with 
\begin{equation}\label{eq:LG}
\left\{\begin{array}{lcl}
L_1^{i,j}(\a) =\frac{\a_{i+1}-\a}{\Delta \a}, 
&&\quad G_1^{i,j}(s)=1-\frac{3(s-s_j)^2}{\Delta s^2}+\frac{2(s-s_j)^3}{\Delta s^3} \\
L_2^{i,j}(\a)=1-L_1^{i,j}(\a),
&&\quad G_2^{i,j}(s)=s-s_j-\frac{2(s-s_j)^2}{\Delta s}+\frac{(s-s_j)^3}{\Delta s^2}\\
&&\quad G_3^{i,j}(s)=1-G_1^{i,j}(s)\\
&&\quad G_4^{i,j}(s)=-G_2^{i,j}(s_j+s_{j+1}-s)
\end{array}\right.
\end{equation}
and that $H_k^{i,j}(\a,s)=0$, $k=1,\ldots,8$, whenever $(\a,s)\not\in C_{i,j}$.% (see also Figure \ref{fig:shape}). 
The basis functions are then defined as:
\begin{equation}\label{basis}
\left\{\begin{array}{r}
\Phi_{i,j} := H_7^{i-1,j-1}+ H_5^{i-1,j} + H_3^{i,j-1} + H_1^{i,j} \\
\Psi_{i,j} :=H_8^{i-1,j-1}+ H_6^{i-1,j} + H_4^{i,j-1} + H_2^{i,j} 
\end{array}\right.
\end{equation}
for $i=1,\ldots,N_\a,\, j=1,\ldots,N_s$, and the element $\vec{F}\in\mathcal V$ can be represented in terms of the point values $\vec{F}_{i,j}$ and the $s$-derivatives $\partial_s \vec{F}_{i,j}$ at the discretization nodes, as:
\begin{equation}\label{eq:I2D}
\vec{F}(\a,s)=\sum_{i=1}^{N_\a} \sum_{j=1}^{N_s} \big( \vec{F}_{i,j} \Phi_{i,j}(\a,s) + \partial_s\vec{F}_{i,j} \Psi_{i,j}(\a,s) \big) \,.
\end{equation}

The FE formulation of the lamellipodium problem on the time interval $[0,T]$ is to find  $\vec{F}\in C^1\big([0,T];\,\mathcal V\big)$, such that (\ref{eq:FEM}) holds for all $\vec{G}\in C\big([0,T];\,\mathcal V\big)$.
